# Supplementary material for: Gigapixel Whole-Slide Images Classification using Locally Supervised Learning
Source: arXiv:2207.08267 ancillary file (2022-09-26)
Supplement: Supplementary file 1 [file Supplementary.pdf]

# Supplementary Material of
# Gigapixel Whole-Slide Images Classification using Locally Supervised Learning

Jingwei Zhang[1⋆], Xin Zhang[1⋆], Ke Ma[2], Rajarsi Gupta[1], Joel Saltz[1], Maria Vakalopoulou[3], and Dimitris Samaras[1]

[1] Stony Brook University, USA
[2] Snap Inc., USA
[3] CentraleSupélec, University of Paris-Saclay, France
{jingwezhang, xin.zhang.3, kemma, samaras}@cs.stonybrook.edu
{Rajarsi.Gupta, Joel.Saltz}@stonybrookmedicine.edu
maria.vakalopoulou@centralesupelec.fr

**Table 1.** Comparison of training seconds per image on three different sized images. Our method was comparable to the end-to-end (E2E) training.

| Image size | $8698 \times 7496$ | $12223 \times 10057$ | $23849 \times 10257$ |
|---|---|---|---|
| E2E | 1.6s | 2.6s | / |
| Ours (K=4) | 1.6s | 3.1s | 6.6s |
| Ours (K=8) | 2.2s | 4.2s | 8.8s |

**Table 2.** Network structures of the reconstruction network $R_i$, the auxiliary classifier $G_i$ and the classifier $H$.

| Reconstruction $R_i$ | Auxiliary classifier $G_i$ | Classifier $H$ |
|---|---|---|
| Bilinear interpolation | Conv2d(kernel_size, stride) | Conv2d($5 \times 5$, $5 \times 5$) |
| Conv2d(3x3, 1x1) | LayerNorm + ReLU | LayerNorm + ReLU |
| BatchNorm + ReLU | GABMIL pooling | GABMIL pooling |
| Conv2d(3x3, 1x1) | Linear(NO. features, 128) | Linear(512, 128) |
| | ReLU | ReLU |
| | Linear(128, NO. classes) | Linear(128, NO. classes) |

⋆ These authors contributed equally to this paper.

**Table 3.** Hyper-parameters used in our experiments. kernel_size and stride are the corresponding values in Table 2.

| Network | | RFR model $U_i$ | | Classifier $A_i$ | |
|---|---|---|---|---|---|
| Hyper-parameters | | No. patches | Patch size | kernel_size | stride |
| K=4 | $G_1$ | 10 | 128 | $9 \times 9$ | $9 \times 9$ |
| | $G_2$ | 10 | 64 | $9 \times 9$ | $9 \times 9$ |
| | $G_3$ | 10 | 32 | $7 \times 7$ | $7 \times 7$ |
| K=8 | $G_1 \sim G_3$ | 10 | 128 | $9 \times 9$ | $9 \times 9$ |
| | $G_4 \sim G_5$ | 10 | 64 | $9 \times 9$ | $9 \times 9$ |
| | $G_6 \sim G_7$ | 10 | 32 | $7 \times 7$ | $7 \times 7$ |

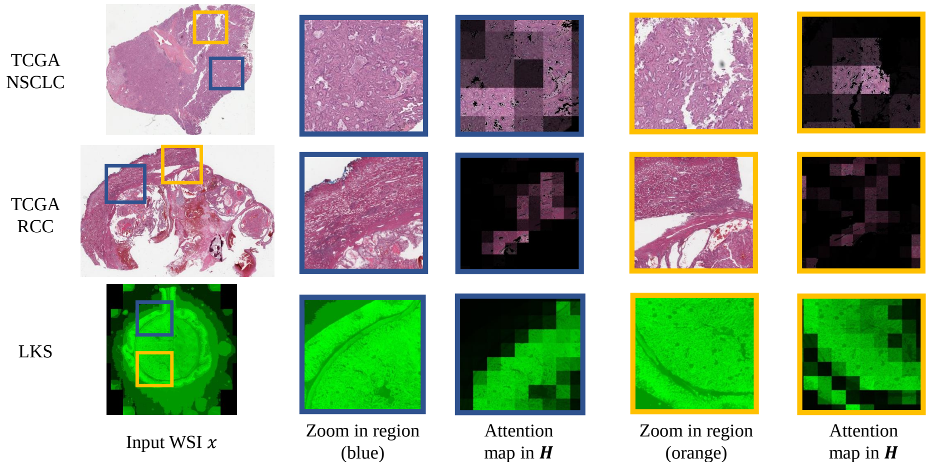


**Fig. 1.** Attention visualization of the GABMIL in the classifier $H(\cdot)$. As the entire image was too large, we picked two regions on each image and showed their local region and attention maps.
